# Supplementary material for: Modern Random Access for Satellite Communications
Source: arXiv:1706.10198 source file (2017-06-30)
Supplement: Supplementary file 1 [file Appendix.tex]

\section*{Appendix - Probability of loops}
