# Supplementary material for: Modern Random Access for Satellite Communications
Source: arXiv:1706.10198 source file (2017-06-30)
Supplement: Supplementary file 2 [file Appendix.tex]

%\section*{Appendix}

%Here we will demonstrate that

%\begin{equation}
%\label{eq:to_demonstrate}
%P_{succ-L3-appr}\leq P_{succ-L3}.
%\end{equation}

%We recall that $P_{succ-L3}=\sum_{i=1}^{\infty} p_i {P_{succ-L2}}^i$ and it can be rewritten as

%\begin{equation}
%\label{eq:exp_exac}
%P_{succ-L3}=\sum_{i=1}^{\infty} p_i {P_{succ-L2}}^i= \mathbb{E}[{P_{succ-L2}}^i],
%\end{equation}

%by definition of expected value for a discrete distribution. Furthermore we can write $P_{succ-L3-appr}$ as

%\[
%P_{succ-L3-appr}=\left(P_{succ-L2}\right)^{\mathbb{E}[\overline{f_X(x)}]}= \left(P_{succ-L2}\right)^{\sum_{i=1}^{\infty}i\cdot p_i},
%\]

%following equations \eqref{eq:P_succ_L3_appr} and \eqref{eq:exp_val}. By definition of expected value for a discrete distribution we can rewrite $P_{succ-L3-appr}$ as

%\begin{equation}
%\label{eq:exp_appr}
%P_{succ-L3-appr}=\left(P_{succ-L2}\right)^{\mathbb{E}[i]}.
%\end{equation}

%In order to demonstrate equation \eqref{eq:to_demonstrate} we can apply the Jensen's inequality \cite{Jensen}. It says that

%\[
%g(\mathbb{E}[i])\leq \mathbb{E}[g(i)],
%\]

%if $g(i)$ is a convex function. In our case $g(i)={P_{succ-L2}}^i$. $g(i)$ is convex if $g''(i)\geq 0$, where $g''(i)$ is the second derivative of $g(i)$. The first derivative of $g(i)$, $g'(i)$ is

%\[
%g'(i)=\frac{d}{di}({P_{succ-L2}}^i)={P_{succ-L2}}^i\log P_{succ-L2}.
%\]

%The second derivative $g''(i)$ is then

%\begin{equation}
%\label{eq:g_second}
%\begin{split}
%g''(i)&=\frac{d}{di}{P_{succ-L2}}^i\log P_{succ-L2}=\\
%&={P_{succ-L2}}^i[\log P_{succ-L2}]^2.
%\end{split}
%\end{equation}

%The first factor in equation \eqref{eq:g_second}, ${P_{succ-L2}}^i$ is ${P_{succ-L2}}^i\geq 0$ for $0\leq P_{succ-L2} \leq 1$ which are the admissible values for a probability and for $i \in \mathbb{N}$. The second factor $[\log P_{succ-L2}]^2$ is $[\log P_{succ-L2}]^2\geq 0$ for $0\leq P_{succ-L2} \leq 1$. So we can conclude that $g''(i)\geq 0$ and therefore $g(i)$ is a convex function. This proves the convexity and therefore, we can write

%\[
%\begin{split}
%P_{succ-L3-appr}&=g(\mathbb{E}[i])=\left(P_{succ-L2}\right)^{\mathbb{E}[i]}\leq\\ &\leq\mathbb{E}[{P_{succ-L2}}^i]=\mathbb{E}[g(i)]=P_{succ-L3}.
%\end{split}
%\]
